# Supplementary material for: A Multimodal Sentiment Dataset for Video Recommendation
Source: arXiv:2109.08333 source file (2021-09-17)
Supplement: Supplementary file 1 [file Appendix.tex]

\documentclass[../acl2021.tex]{subfiles}

\begin{document}

\end{document}
